# Supplementary material for: Quantum Bisimilarity is a Congruence under Physically Admissible Schedulers
Source: arXiv:2408.15087 source file (2024-08-27)
Supplement: Supplementary file 1 [file appendix_assessment.tex]

\subsection{Proof of \autoref{thm:probsmallerthanconst}}
To prove \autoref{thm:probsmallerthanconst} we need to introduce tagged processes. The idea is that whenever a distribution $O[\Delta]$ can perform an indexed transition $\longsquiggly_\pi$, then the tagged version $\ptag{O[\Delta]}$ express a barb named $\pi$ with probability one. This allows us to interpret the enhanced semantics as standard probabilistic reductions, and show that constrained saturated bisimilarity does not have greater discriminating power (thanks to indices) with respect to saturated bisimilarity.

\begin{definition}[Tagging operation]
	We define the $\ptag{\blank}_k^\pi$ operation, which tags (the observer in a) configuration with barbs in $\{\ell, r, \iota\}^*$. $k$ is the starting string of the barb, and $\pi$ is used when we want to add an additional $\iota$ in front of the barbs starting with $\pi$
	\begin{align*}
		\ptag{\conf{\rho, P, R}}^\pi_k   & = \conf{\rho, P \parallel \ptag{R}^\pi_k}
		                                 &                                                &  & \ptag{\bot}^\pi_k              & = \bot
		\\
		\ptag{P \parallel Q}^{\ell\pi}_k & = \ptag{P}^\pi_{k\ell} \parallel \ptag{Q}_{kr}
		                                 &                                                &  & \ptag{P \parallel Q}^{r\pi}_k  & = \ptag{P}_{k\ell} \parallel \ptag{Q}^{\pi}_{kr}
		\\
		\ptag{P}^\varepsilon_k           & = \ptag{P}_{k\barr}
		                                 &                                                &  & \ptag{\nil_{\tilde e}}_k       & = \nil_{\tilde e}
		\\
		\ptag{\sop{E}{\tilde{x}}.P}_k    & = \sop{E}{\tilde{x}}.\ptag{P}_{k\iota} + k!0
		                                 &                                                &  & \ptag{\meas{\tilde{x}}{y}.P}_k & = \meas{\tilde{x}}{y}.\ptag{P}_{k\iota} + k!0
		\\
		\ptag{c?x.P}_k                   & = c?x.\ptag{P}_{k\iota} + k!0
		                                 &                                                &  & \ptag{c!e}_k                   & = c!e + k!0
		\\
		\ptag{P + Q}_k                   & = \ptag{P}_k + \ptag{Q}_k
		                                 &                                                &  & \ptag{\ite{e}{P}{Q}}_k         & = \ite{e}{\ptag{P}_k}{\ptag{Q}_k}
	\end{align*}
	We extend the tagging operation via linearity: $\ptag{\Delta_1 \psum{p} \Delta_2}_k^\pi = \ptag{\Delta_1}_k^\pi \psum{p} \ptag{\Delta_2}_k^\pi$. We will often write $\ptag{\blank}$ instead of $\ptag{\blank}_\varepsilon$.
\end{definition}

\begin{definition}[Tagged transitions]
	We define the set of tags a configuration \[T(\iconf) = \{\pi \in \{l, r, \barr\}^* \mid \iconf\downarrow_\pi\}\]
	We define two kinds of tagged transition from (tagged) configurations to distributions
	\begin{align*}
		\ptag{\iconf} \tauarrow \Delta : \diamond \qquad & \text{iff } T(\ptag{\iconf}) = T(\ptag{\iconf'}) \ \forall \ptag{\iconf'} \in \lceil \Delta \rceil                                                                                                           \\
		\ptag{\iconf} \tauarrow \Delta : \lambda \qquad  & \text{iff } \lambda \in T(\ptag{\iconf}) \text{ and } \lambda \not\in T(\ptag{\iconf'}),  T(\ptag{\iconf})\setminus\{\lambda\} \subseteq T(\ptag{\iconf'}) \ \forall \ptag{\iconf'} \in \lceil \Delta \rceil
	\end{align*}
	And we extend this notion to distributions via linearity
	\[
		\ptag{\Delta_1} \psum{p} \ptag{\Delta_2} \tauarrow \Delta'_1 \psum{p} \Delta'_2 : \pi  \text{ if and only if } \ptag{\Delta_i} \tauarrow \Delta_i : \pi \text{ for } i \in {1, 2}
	\]
\end{definition}

We now prove that the indexed transitions of $\conf{\rho, P, R}$ are essentially the same of the tagged transitions of $\ptag{\conf{\rho, P, R}}$.

\begin{lemma}\label{interpretdiamond}
	For any observer $R$ we have
	\[
		\forall k \ \left(
		\conf{\rho, P, R} \longsquiggly_\diamond \Delta
		\Longleftrightarrow
		\conf{\rho, P \parallel \ptag{R}_k}  \tauarrow \Delta' : \diamond	\text{ with } \ptag{\Delta}_k \equiv \Delta'
		\right)\]
\end{lemma}
\begin{proof}
	The proof follows easily from the definition of $\diamond$-tagged transitions.
\end{proof}

\begin{lemma}\label{interpretfw} %
  For any observer $R$ and index $\lambda \neq \diamond$, we have
  \[
    \forall k \ldotp \conf{\rho, P, R} \longsquiggly_\lambda \Delta \Longrightarrow
    \conf{\rho, P \parallel \ptag{R}_k} \to \ptag{\Delta}^\lambda_k : k\lambda
  \]
\end{lemma}
\begin{proof}
  We will proceed by induction on the transition $\longsquiggly_\lambda$.

  If rule \textsc{OQOp} is valid, then $R \equiv \sop{E}{\tilde{q}}.R_1$, we
  have
  \[
    \iconf = \conf{\rho, P, \sop{E}{\tilde{q}}.R_1} \longsquiggly_\varepsilon
    \sconf{\mathcal{E}_{\tilde{q}}(\rho), P, R_1} = \Delta
  \]
  and
  \[
    \ptag{\iconf}_k =
    \conf{\rho, P \parallel (\sop{E}{\tilde{q}}.\ptag{R_1}_{k\barr} +
    k!0)}
    \to \sconf{\mathcal{E}_{\tilde{q}}(\rho), P \parallel \ptag{R_1}_{k\barr}} =
    \ptag{\Delta}^\varepsilon_k
  \]
  We must further check that:
  $\ptag{\iconf}_k \to \ptag{\Delta}^\varepsilon_k :
  k$. The first condition, $k \in T(\ptag{\iconf}_k)$, is true by $k!0$.
  The second, $k \not\in T(\iconf')$, is true because any new barb expressed by $\ptag{R_1}_{k\barr}$ must start with
  $k\barr$. The third condition, $T(\ptag{\iconf}_k) \setminus \{k\} \subseteq
  T(\ptag{\Delta}^\varepsilon_k)$, is also trivially true since the only syntactic difference between the $\iconf$ and
  $\Delta$ is the barb-expressing $k!0$.

  If rule \textsc{OQMeas} is valid, then $R \equiv \meas{\tilde{q}}{y}.R_1$, we
  have
  \[
    \iconf = \conf{\rho, P, \meas{\tilde{q}}{y}.R_1} \longsquiggly_\varepsilon
    \sum_{i=0}^{|M| - 1}\distelem{p_m}{\sconf{\frac{\rho_m}{p_m}, P, R_1[\sfrac{m}{y}]}} = \Delta
  \]
  and, noting as before that $\ptag{R[\sfrac{v}{x}]}^\lambda_k =
  \ptag{R}^\lambda_k[\sfrac{v}{x}]$
  \[
    \ptag{\iconf}_k
    = \conf{\rho, P \parallel (\meas{\tilde{q}}{y}.\ptag{R_1}_{k\barr} +
    k!0)}
    \to \sum_{i=0}^{|M| - 1}\distelem{p_m}{\sconf{\frac{\rho_m}{p_m}, P \parallel
    (\ptag{R_1}_{k\barr}[\sfrac{m}{y}] + k!0)}} =
    \ptag{\Delta}^\varepsilon_k
  \]
  $\ptag{\iconf}_k \to \ptag{\Delta}^\varepsilon_k :
  k$ holds as for the \textsc{OQOp} noting that each element in
  $\ptag{\Delta}^\varepsilon_k$ has syntactically the same sendings.

  If rule \textsc{Input} is valid, then $R \equiv c?x.R_1 + R_2$, we have
  \[
    \iconf =
    \conf{\rho, (c!v + P_1) \parallel P_2 \setminus D, c?x.R_1 + R_2} 
    \longsquiggly_\varepsilon \sconf{\rho, P_2 \setminus D, R_1[\sfrac{v}{x}]}
    = \Delta
  \]
  and
  \begin{align*}
    \ptag{\iconf}_k
    &= \conf{\rho, ((c!v + P_1) \parallel P_2 \setminus D) \parallel (c?x.\ptag{R_1}_{k\barr} + k!0 + \ptag{R_2}_k)} \\
    &\equiv \conf{\rho, ((c!v + P_1) \parallel P_2 \parallel (c?x.\ptag{R_1}_{k\barr} + k!0 + \ptag{R_2}_k)) \setminus D} \\
    &\to \sconf{\rho, (P_2 \parallel \ptag{R_1}_{k\barr}[\sfrac{v}{x}]) \setminus D} \\
    &\equiv \sconf{\rho, (P_2 \setminus D) \parallel \ptag{R_1[\sfrac{v}{x}]}_{k\barr}}
    = \ptag{\Delta}^\varepsilon_k
  \end{align*}
  $\ptag{\iconf}_k \to \ptag{\Delta}^\varepsilon_k :
  k$ holds trivially as for the \textsc{OQOp}.

  If rule \textsc{Output} is valid, then $R \equiv c!v$, we have
  \[
    \iconf =
    \conf{\rho, (c?x.P_1) + P_2) \parallel P_3 \setminus D, c!v} 
    \longsquiggly_\varepsilon \sconf{\rho, (P_1[\sfrac{v}{x}] \parallel P_3) \setminus D, \nil}
    = \Delta
  \]
  and
  \begin{align*}
    \ptag{\iconf}_k
    &= \conf{\rho, (((c?x.P_1) + P_2) \parallel P_3 \setminus D) \parallel (c!v + k!0)} \\
    &\equiv \conf{\rho, (((c?x.P_1) + P_2) \parallel P_3 \parallel (c!v + k!0)) \setminus D} \\
    &\to \sconf{\rho, (P_1[\sfrac{v}{x}] \parallel P_3 \parallel \nil) \setminus D} \\
    &\equiv \sconf{\rho, (P_1[\sfrac{v}{x}] \parallel P_3 \setminus D) \parallel \nil}
    = \ptag{\Delta}^\varepsilon_k
  \end{align*}
  $\ptag{\iconf}_k \to \ptag{\Delta}^\varepsilon_k :
  k$ holds trivially as for the \textsc{QInput}.

  If rule \textsc{ParL} is valid, then $R \equiv R_1 \parallel R_2$, we have
  \[
    \iconf =
    \conf{\rho, P, R_1 \parallel R_2}
    \longsquiggly_{\ell\lambda} \Theta \parallel R_2
    = \Delta
  \]
  By inductive hypothesis, for any $k$
  \[
    \conf{\rho, P, R_1} \longsquiggly_\lambda \Theta \Longrightarrow \conf{\rho, P \parallel \ptag{R_1}_k} \to \ptag{\Theta}^\lambda_k : k\lambda
  \]
  and
  \begin{align*}
    \ptag{\iconf}_k
    = \conf{\rho, P \parallel \ptag{R_1}_{k\ell} \parallel \ptag{R_2}_{kr}}
    \to \ptag{\Theta}^\lambda_{k\ell} \parallel \ptag{R_2}_{kr}
    = \ptag{\Delta}^{\ell\lambda}_k
  \end{align*}
  $\ptag{\iconf}_k \to \ptag{\Delta}^{\ell\lambda}_k : k\ell\lambda$ holds by inductive hypothesis by setting $k = k\ell$.
  The case for \textsc{ParR} is analogous to the case for \textsc{ParL}.

  Finally, the \textsc{Congr} rule is simply resolved by induction, since its trivial to show that the congruence relation does not change the barbs expressed by a distribution.
\end{proof}

\begin{lemma}\label{interpretbw} %
	For any observer $R$ and index $\lambda \neq \diamond$, we have
	\[\forall k \ \left( \conf{\rho, P \parallel \ptag{R}_k}  \rightarrow \Delta : k\lambda
	\Longrightarrow	
	\conf{\rho, P, R} \longsquiggly_\lambda \Delta' \text{ with } \ptag{\Delta'}_k^{\lambda} \equiv \Delta
	\right)\]
\end{lemma}
\begin{proof}

Note that any transition $\ptag{\mathcal{C}}_k = \conf{\rho, P \parallel \ptag{R}_k}  \rightarrow \Delta : k\lambda$ must involve $R$, because a transition modifying only $P$ would not be tagged as $k\lambda$. We will then proceed on induction on the syntax of $R$.

If $R = \nil_{\tilde{e}}$, there are no $k\lambda$-tagged transitions going out from $\ptag{\conf{\rho, P\parallel \nil_{\tilde{e}}}} =  \conf{\rho, P\parallel \nil_{\tilde{e}}}$.

If $R = \sop{E}{\tilde{x}}.R' $, we have \[\ptag{\mathcal{C}}_k \equiv \conf{\rho, P \parallel \sop{E}{\tilde{x}}.\ptag{R'}_{k\barr} + k!0} \rightarrow \Delta \equiv \singleton{\conf{\sop[\tilde{e}]{E}{\rho}, P \parallel \ptag{R'}_{k\barr}}}~:~k\]
But then 
\begin{align*}
&\conf{\rho, P, \sop{E}{\tilde{x}}.R'} \longsquiggly_\varepsilon \Delta' = \singleton{\conf{\sop[\tilde{e}]{E}{\rho}, P, R'}}, \text{ and }\\
&\ptag{\Delta'}_k^{\varepsilon} = \singleton{\conf{\sop[\tilde{e}]{E}{\rho}, P \parallel \ptag{R'}_{k}^{\varepsilon}}} = \singleton{\conf{\sop[\tilde{e}]{E}{\rho}, P \parallel \ptag{R'}_{k\barr}}} \equiv \Delta.
\end{align*}

If $R = \meas{\tilde{x}}{y}.R'$, we have
\[\conf{\rho, P \parallel \meas{\tilde{x}}{y}.\ptag{R'}_{k\barr} + \varepsilon!0} \rightarrow \Delta \equiv \sum_m \distelem{p_m}{\singleton{\conf{\rho_m, P \parallel \ptag{R'}_{k\barr}[m/y]}}} : \varepsilon\]
for some set of $p_m$ and $\rho_m$. Then the proof is identical to the previous case, noticing that $\ptag{R[v/x]}_k^\lambda = \ptag{R}_k^\lambda[v/x]$ as the tags depends on the position of the processes and not on their content.

If $R = c!e $, then $P$ must be receiving on the unrestricted channel $c$, so we have \[\ptag{\mathcal{C}}_k \equiv \conf{\rho, (((c?x.P') + P'') \parallel Q \parallel (c!v + \varepsilon!0)) \setminus D} \rightarrow \Delta \equiv \singleton{\conf{\rho, ( P'[v/x] \parallel Q )\setminus D}}~:~\varepsilon\]
for some (possibly empty) set of restrictions $D$ and processes $P', P'', Q$. But then \\ $\mathcal{C} \equiv_o \conf{\rho, (((c?x.P') + P'') \parallel Q)  \setminus D, c!v} \longsquiggly_\varepsilon \Delta' = \singleton{\conf{\rho, ( P'[v/x] \parallel Q )\setminus D, \nil}}$ and $\ptag{\Delta'}_k^{\varepsilon} \equiv \Delta$.

If $R$ is a sum of reception, then $P$ must be sending on at least one of the channel in $R$, so we have 
\[\ptag{\mathcal{C}}_k \equiv \conf{\rho, (((c!v + P) \parallel Q \parallel (c?x.\ptag{R'}_{k\barr} + \ptag{T}_k + \varepsilon!0)) \setminus D} \rightarrow \Delta \equiv \singleton{\conf{\rho, ( Q \setminus D )\parallel R'[v/x]}}~:~\varepsilon\]
for some (possibly empty) set of restrictions $D$ and process $Q$, and the proof is identical to the previous case.

If $R = \ite{e}{R_1}{R_2}$, then the only way to have a transition is after applying the structural congruence and obtaining either $R_1$ or $R_2$, from which the desired property is obtained thanks to the inductive hypothesis and the fact that $\ptag{R}_k \equiv \ptag{R'}_k$ if and only if $R \equiv_o R'$.

If $R =  R_1 \expar R_2 $ and $\ptag{\mathcal{C}}_k \equiv \conf{\rho, P \parallel \ptag{R_1}_{kl} \parallel \ptag{R_2}_{kr}} \rightarrow \Delta : k\lambda$, then the transition cannot be a synchronisation between $R_1$ and $R_2$ because all the tags of $\ptag{C}_k$ must be in $\Delta$ except from $k\lambda$, and a synchronisation would destroy two tags, not just one. Suppose then that the transition involves $R_1$, the $R_2$ case is symmetric. From the $\rulename{SemPar}$ rule must be $\conf{\rho, P \parallel \ptag{R_1}_{k\ell}} \rightarrow \Delta_\ell$ with $\Delta = \Delta_\ell \parallel\ptag{R_2}_{kr} $.  This transition is still tagged with $k\lambda$, as the $k\lambda$ tag is present in $\ptag{R_1}_{k\ell} \parallel \ptag{R_2}_{kr}$ but is absent in $\Delta_\ell \parallel\ptag{R_2}_{kr}$, no must be in $\ptag{R_1}_{kl}$. Besides, we know that $k\lambda = k\ell\lambda'$ for some $\lambda'$, as it is easy to verify that all the tags in $\ptag{R_1}_{k\ell}$ start with $k\ell$. Then we can apply the inductive hypothesis 
\begin{gather*}
\conf{\rho, P \parallel \ptag{R_1}_{k\ell}} \rightarrow \Delta_\ell :k\ell\lambda' 
\qquad \Rightarrow  \qquad
\conf{\rho, P, R_1} \longsquiggly_{\lambda'} \Delta_\ell' \text{ with } \ptag{\Delta_\ell'}_{k\ell}^{\lambda'} = \Delta_\ell
\end{gather*}
and derive 
\[\conf{\rho, P, R_1 \expar R_2} \longsquiggly_{\lambda} \Delta' = \Delta_\ell'\parallel R_2 \text{ with } \ptag{\Delta'}_k^{\lambda} = \Delta
\]
since $\lambda = \ell\lambda'$ and $\ptag{\Delta'}_k^{\lambda} = \ptag{\Delta_\ell'\parallel R_2}_k^{\ell\lambda'} = \ptag{\Delta_\ell'}_{k\ell}^{\lambda'} \parallel \ptag{R_2}_{kr}  = \Delta_\ell \parallel \ptag{R_2}_{kr} = \Delta$.
\end{proof}

\begin{lemma}\label{interpretdistr}
	For any $\Delta, \Delta'$ that do not contain $\bot$, we have
	\[
		\forall k \ \left(
		\Delta \longsquiggly_\pi \Delta'
		\Longleftrightarrow
		\ptag{\Delta}  \tauarrow \Delta'' : \pi	\text{ with } \ptag{\Delta'}_k \equiv \Delta''
		\right)\]
\end{lemma}
\begin{proof}
	The proof follows from \autoref{interpretdiamond}, \autoref{interpretfw} and \autoref{interpretbw}, thanks to linearity of $\longsquiggly_\pi$ and $\tauarrow~:~\pi$
\end{proof}

We can now finally prove \autoref{thm:probsmallerthanconst}

\probsmallerthanconst*
\begin{proof}
	The direction $\sim_{cs} \not\subseteq \sim_{s}$ is given by \autoref{ex:zopm}.
	For $\sim_{s} \subseteq \sim_{cs}$, we define the relation $\rel = \{(\Delta, \Theta) \mid \ptag{\Delta} \sim_{s} \ptag{\Theta}\} $
	And then we prove that $\rel$ is a constrained distribution bisimulation. Notice that, taken $\Delta, \Theta \in \sim_{s}$, when we interpret them as distribution of triples they have a $\nil$ observer, and so $\ptag{\Delta} = \Delta$ and $\ptag{\Theta} = \Theta$. This means that $\sim_{s} \subseteq \rel$, and if $\rel$ is a bisimulation then $\sim_s \subseteq \sim_{cs}$.
	Notice also that $\rel$ is context-closed, meaning that if $\Delta, \Theta \in \rel$, then also $O[\Delta], O[\Theta] \in \rel$ for any $O[\blank]$, because $\sim_s$ is context-closed. Finally, $\rel$ is linear and decomposable, as $\ptag{\blank}$ is defined by linearity and $\sim_s$ is linear and decomposable (as proven in~\cite{hennessyexploring2012}, proposition 5.8).

	Take $\Delta, \Theta \in \rel$. Since $\ptag{\Delta}$ and $\ptag{\Theta}$ are bisimilar, they express the same barbs. But $\ptag{\Delta}$ expresses at least all the barbs of $\Delta$ (and similarly $\ptag{\Theta}$), so also $\Delta$ and $\Theta$ must express the same barbs.

	Suppose $\Delta \longsquiggly_\pi \Delta'$, we will prove that there exists a transition $\Theta \longsquiggly_\pi \Theta'$ with $\Delta' \rel \Theta'$, the other direction is symmetric. Let $\Delta' = \Delta'_{\not\bot} \psum{p} \singleton{\bot}$, where $\Delta'_{\not\bot}$ does not contain $\bot$.  Then, by decomposability of $\longsquiggly_\pi$ and of $\rel$, it must be $\Delta = \Delta_{\not\bot} \psum{p} \Delta_\bot$, and also $\Theta = \Theta_{\not\bot} \psum{p} \Theta\bot$. Since $\Delta_\bot \longsquiggly_\pi \bot$, from \autoref{interpretdistr} it follows that there is no $\Delta'$ such that $\ptag{\Delta_\bot} \tauarrow \Delta'~:~\pi$. But since $\ptag{\Delta_\bot} \sim_{s} \ptag{\Theta_\bot}$, using the third property of bisimilarity (from $\Theta$ to $\Delta$) we get that there is no  $\Theta'$ either such that $\ptag{\Theta_\bot} \tauarrow \Theta'~:~\pi$. Then, from \autoref{interpretdistr} it follows that $\Theta_\bot \longsquiggly_\pi \bot$, and of course $(\bot, \bot) \in \rel$.

	Consider now $\Delta_{\not\bot}$. From $\Delta_{\not\bot} \longsquiggly_\pi \Delta'_{\not\bot}$, we know that $\ptag{\Delta_{\not\bot}} \tauarrow \ptag{\Delta'_{\not\bot}}^\pi~:~\pi$ tanks to \autoref{interpretdistr}, and so
	$\ptag{\Theta_{\not\bot}} \tauarrow \Theta'$ for a $\Theta' \sim_{s} \ptag{\Delta'_{\not\bot}}^\pi$. But since they are bisimilar, they express the same barbs, and from $\ptag{\Theta_{\not\bot}} \tauarrow \Theta'~:~\pi$ we
	get $\Theta_{\not\bot} \longsquiggly_\pi \Theta''$ with $\ptag{\Theta''}^\pi \equiv \Theta'$.
	To sum up, we have
	\[
		\begin{matrix}%
			\Delta = \Delta_{\not\bot} \psum{p} \Delta_{\bot} &
			\rel                                              &
			\Theta = \Theta_{\not\bot} \psum{p} \Theta{\bot}                           \\
			\downsquiggly[\pi]                                &   & \downsquiggly[\pi] \\
			\Delta' = \Delta'_{\not\bot} \psum{p} \bot        &
			?                                                 &
			\Theta' = \Theta'' \psum{p} \bot
		\end{matrix}
	\]
	with $\ptag{\Delta'_{\not\bot}}^\pi \sim_{s} \ptag{\Theta''}^\pi$. It's possible to verify that $\ptag{\Delta}^\pi \sim_{s} \ptag{\Theta}^\pi$ implies $\ptag{\Delta} \sim_{s} \ptag{\Theta}$, as there is a bijection $f$ between the free channels of $\ptag{\Delta}$ and of $\ptag{\Delta}^\pi$, and so any context $O[\blank]$ applied on $\ptag{\Delta}$ has the same behaviour of the context $f(O[\blank])$ applied on $\ptag{\Delta}^\pi$, and vice versa. Given that, since $\bot, \bot \in \rel$ and $\rel$ is linear, we can conclude $\Delta' \rel \Theta'$.
\end{proof}

\subsection{Proof of \autoref{thm:linearity} and \autoref{thm:propertyA}}\label{uptoappendix}

Before proving \autoref{thm:linearity} and \autoref{thm:propertyA}, it is convenient to prove the soundness of the bisimilarity up to convex hull technique~\cite{bonchipower2017}.
To do so, let us define the function on relations $b$, which is the function of which bisimilarity is the greatest fix point
\begin{footnotesize}
	\[
		b(\rel) \coloneqq \left\{
		(\Delta, \Theta) \biggm| \begin{array}{c}
			\Delta \downarrow_{b}^p \Leftrightarrow \Theta \downarrow_{b}^p \\
			O[\Delta] \longsquiggly_\pi \Delta' \Rightarrow \exists \Theta' \ O[\Theta] \longsquiggly_\pi \Theta' \wedge \Delta'\,\rel\,\Theta'
			\\
			O[\Theta] \longsquiggly_\pi \Theta' \Rightarrow \exists \Delta' \ O[\Delta] \longsquiggly_\pi \Delta' \wedge \Delta'\,\rel\,\Theta'
		\end{array}
		\right\}
	\]
\end{footnotesize}

and recall the definition of convex hull from~\cite{bonchipower2017}
\[
	Cv(\rel) \coloneqq \bigg\{\bigg(\sum_{i \in I} \distelem{p_i}{\Delta_i}, \sum_{i \in I} \distelem{p_i}{\Theta_i}\bigg)\ \bigg|\ \forall i \in I \ldotp \Delta_i\,\rel\,\Theta_i \bigg\}
\]

Observe that both $b$ and $Cv$ are monotone functions on the lattice of relations.

\begin{lemma}[$Cv$ is $b$-compatible]\label{thm:cvcomp}
	We have that $\forall \rel\ldotp Cv(b(\rel)) \subseteq b(Cv(\rel))$.
\end{lemma}
\begin{proof}
	Assume $(\Delta, \Theta) \in Cv(b(\rel))$. Then it must be $\Delta = \sum_{i \in I}\distelem{p_i} \Delta_i$ and $\Theta = \sum_{i \in I}\distelem{p_i} \Theta_i$ for a certain set of probabilities $\{p_i\}_{i \in I}$, with
	$\Delta_i\,b(\rel)\,\Theta_i$. So we have, for any $i \in I$
	\begin{gather*}
		\sum_{\mathcal{C} \downarrow_c} \Delta_i(\mathcal{C}) = \sum_{\mathcal{C} \downarrow_c} \Theta_i(\mathcal{C}) = q_i \\
		\sum_{\mathcal{C} \downarrow_c} \sum_{i \in I} p_i \Delta_i(\mathcal{C})  =
		\sum_{\mathcal{C} \downarrow_c} \sum_{i \in I} p_i \Theta_i(\mathcal{C}) = \sum_{i \in I} p_i q_i = q
	\end{gather*}
	meaning that $\Delta \downarrow_c^q$ if and only if $\Theta \downarrow_c^q$. The same holds also for $\Delta \downarrow_\bot^q$ and $\Theta \downarrow_\bot^q$, as
	\begin{gather*}
		\Delta_i(\bot) = \Theta_i(\bot) = q_i \\
		\sum_{i \in I} p_i \Delta_i(\bot)  =
		\sum_{i \in I} p_i \Theta_i(\bot) = \sum_{i \in I} p_i q_i = q
	\end{gather*}

	Suppose $O[\Delta] = \sum_{i \in I} \distelem{p_i} O[\Delta_i]  \longsquiggly_\pi \Delta'$.
	From~\cite{hennessyexploring2012}, $\longsquiggly_\pi$ is left-decomposable, so it must be $\Delta'
		= \sum_{i \in I} \distelem{p_i} \Delta_i'$ with $O[\Delta_i] \longsquiggly_\pi\Delta_i'$. But
	since $\Delta_i\,b(\rel)\,\Theta_i$ it must be $O[\Theta_i] \longsquiggly_\pi
		\Theta_i'$ with $\Delta_i'\,\rel\,\Theta_i'$ for any $i \in I$, from which it follows that
	$\sum_{i \in I} \distelem{p_i} O[\Theta_i] \longsquiggly_\pi \sum_{i \in I} \distelem{p_i} \Theta_i' = \Theta'$.

	In other words, $\Delta$ and $\Theta$ express the same barbs and whenever
	$O[\Delta] \longsquiggly_\pi \Delta'$, there exists a transition $O[\Theta]
		\longsquiggly_\pi \Theta'$ such that $\Delta'\,Cv(\rel)\,\Theta'$ (the symmetrical
	argument is the same). So we can conclude that $(\Delta, \Theta) \in
		b(Cv(\rel))$.
\end{proof}

From~\cite{sangiorgienhancements2011}, we know that if $Cv$ is compatible, then bisimulations up to $Cv$ are a sound proof technique.
Besides, it also allows us to show linearity of $\sim_{cs}$ as a corollary (note that the same proof holds also for $\sim_s$).

\linearity*
\begin{proof}
	We can easily prove that $Cv(\sim_{cs}) \subseteq\ \sim_{cs}$. Since $Cv$ is
	$b$-compatible, we have that $Cv(b(\sim_{cs})) \subseteq b(Cv(\sim_{cs}))$, and
	since $\sim_{cs}$ is the greatest fix point of $b$, we have $Cv(\sim_{cs}) \subseteq
		b(Cv(\sim_{cs}))$, meaning that $Cv(\sim_{cs})$ is a bisimulation, and so
	$Cv(\sim_{cs}) \subseteq\ \sim_{cs}$.
\end{proof}

In order to prove \autoref{thm:propertyA}, we first need a lemma on deterministic distributions.

\begin{lemma}\label{sum of deterministic is deterministic}
	If $\Delta, \Theta$ are deterministic, then $\Delta \psum{p} \Theta$ is deterministic for each probability $p$.
\end{lemma}
\begin{proof}
	We will prove that, for any probability $p$
	\[
		\mathcal{A} = \left\{  \Delta \psum{p} \Theta \mid \Delta, \Theta \text { are deterministic}\right\}
	\]
	is a deterministic set.
	If $(\Delta \psum{p} \Theta) \longsquiggly_\pi \Xi'$, and $(\Delta \psum{p} \Theta) \longsquiggly_\pi \Xi''$, since $\longsquiggly_\pi$ is decomposable it must be $\Xi' = \Delta' \psum{p} \Theta'$ and $\Xi'' = \Delta'' \psum{p} \Theta''$, with $\Delta \longsquiggly_\pi \Delta'$, $\Delta \longsquiggly_\pi \Delta''$, $\Theta \longsquiggly_\pi \Theta'$ and $\Theta \longsquiggly_\pi \Theta''$. But then, since $\Delta$ and $\Theta$ are deterministic, we have $\Delta' \sim_{cs} \Delta''$, $\Theta' \sim_{cs} \Theta''$ and they are all deterministic, so $\Xi', \Xi'' \in \mathcal{A}$ and $\Xi'\sim_{cs} \Xi''$, for linearity of $\sim_{cs}$.
\end{proof}

\propertyA*
\begin{proof}
	For any deterministic $P$, we define
	\[
		\rel' = \left\{ \left(\singleton{\conf{\rho \psum{p} \sigma, P, R}} \ , \ \singleton{\conf{\rho, P, R}} \psum{p} \singleton{\conf{\sigma, P, R}}\right) \mid \rho, \sigma, p, R \right\}
	\]
	and prove that $\rel = \rel' \cup \{(\bot, \bot)\}$ is a bisimulation up to $Cv$ and up to bisimilarity. That is, we require that if $\Delta \longsquiggly_\pi \Delta'$ then $\Theta \longsquiggly_\pi \Theta'$ with $\Delta' \sim_{cs} Cv(\rel) \sim_{cs} \Theta'$.
	Since $Cv$ is compatible, bisimulation up to $Cv$ and up to bisimilarity is a valid proof technique~\cite{sangiorgienhancements2011}.

	The case $\Delta = \Theta = \bot$ is straightforward. Otherwise, let $\Delta = \singleton{\conf{\nu, P, R}}, \Theta = \singleton{\conf{\rho, P, R}} \psum{p} \singleton{\conf{\sigma, P, R}}$ be in $\rel$, with $\nu = \rho \psum{p} \sigma$. Since they have the same process and observer, they are typed by the same context $\Sigma$. Notice that we do not need to quantify over any context $O[\blank]$, because  $\rel$ is a saturated relation, meaning that if $\Delta, \Theta \in \rel$, then $O[\Delta], O[\Theta] \in \rel$ for any context.

	For the first condition, we have that $\Delta\downarrow_c^p$ if and only if $p = 1$ and $P$ or $R$ express the barb $c$. Then, also $\Theta$ expresses the barb $c$ with probability one, and vice versa.

	For the second condition, suppose that $\singleton{\conf{\nu, P, R}} \longsquiggly_\pi \Delta'$. We will proceed by induction on $\longsquiggly_\pi$ to prove that $\Theta \longsquiggly_\pi \Theta'$ with $\Delta' Cv(\rel) \Theta'$. The ``classical'' cases, that do not modify the quantum state, are trivial, since if $\Delta \longsquiggly_\pi \Delta'$ then $\Theta$ can go in $\Theta'$ performing the same move in both configurations, and $\Delta' \rel \Theta'$. The only interesting cases are $\textsc{QOp}$ and $\textsc{QMeas}$ for the process, and  $\textsc{OQOp}$ and $\textsc{OQMeas}$ for the observer.

	In the $\rulename{QOp}$ case, if
	\[\singleton{\conf{\nu, \sop{E}{\tilde{x}}.P', R}} \longsquiggly_\diamond \singleton{\conf{\sop[\tilde{x}]{E}{\nu}, P', R}}\]
	then
	\begin{gather*}
		\singleton{\conf{\rho, \sop{E}{\tilde{x}}.P', R}} \psum{p} \singleton{\conf{\sigma, \sop{E}{\tilde{x}}.P', R}}\ \longsquiggly_{\diamond}\ \singleton{\conf{\sop[\tilde{x}]{E}{\rho}, P', R}} \psum{p} \singleton{\conf{\sop[\tilde{x}]{E}{\sigma}, P', R}}
	\end{gather*}
	and $\sop[\tilde{x}]{E}{\rho} \psum{p} \sop[\tilde{x}]{E}{\sigma} = \sop[\tilde{x}]{E}{\rho \psum{p} \sigma} = \sop[\tilde{x}]{E}{\nu}$, thanks to linearity of superoperators. The $\rulename{OQOp}$ case is identical.

	In the $\rulename{QMeas}$ case, we have
	\[ \singleton{\conf{\nu, \meas{\tilde{x}}{y}.P', R}} \longsquiggly_\diamond  \Delta' \]
	with
	\[\Delta' = \sum_m \distelem{tr_m(\nu)}\singleton{\conf{\nu'_m, P'[\sfrac{m}{y}], R}} \qquad \nu'_m = \frac{\sop[m]{M}{\nu}}{tr_m(\nu)}
	\]
	where $\sop[m]{M}{\nu} = (M_m\otimes I) \nu (M_m\otimes I)^\dagger$ is the trace-nonincreasing superoperator corresponding to outcome $m$ when measuring qubits $\tilde{x}$, and $tr_m{\nu} = tr(\sop[m]{M}{\nu})$ is the probability of said outcome.
	Then
	\[
		\singleton{\conf{\rho, \meas{\tilde{x}}{y}.P', R}} \psum{p} \singleton{\conf{\sigma, \meas{\tilde{x}}{y}.P', R}}
		\longsquiggly_\diamond \Theta'_\rho \psum{p} \Theta'_\sigma
	\]
	with
	\begin{align*}
		\Theta'_\rho   & = \sum_m \distelem{tr_m(\rho)} \singleton{\conf{\rho'_m, P'[\sfrac{m}{y}], R}} \qquad \rho'_m = \frac{\sop[m]{M}{\rho}}{tr_m(\rho)}
		\\
		\Theta'_\sigma & = \sum_m \distelem{tr_m(\sigma)} \singleton{\conf{\sigma'_m, P'[\sfrac{m}{y}], R}} \qquad \sigma'_m = \frac{\sop[m]{M}{\sigma}}{tr_m(\sigma)}
	\end{align*}
	Observe that $tr_m(\nu) = tr(\sop[m]{M}{\rho \psum{p} \sigma})$ is equal to $tr_m(\rho) \psum{p} tr_m(\sigma)$, thanks to linearity of superoperators and trace. So, according to the rules of probability distributions, $\Theta'_\rho \psum{p} \Theta'_\sigma$ can be rewritten as
	\[
		\sum_m \distelem{tr_m(\nu)} (\singleton{\conf{\rho'_m, P'[\sfrac{m}{y}], R}} \psum{q} \singleton{\conf{\sigma'_m, P'[\sfrac{m}{y}], R}})
	\]
	with $q = \frac{p\cdot tr_m(\rho)}{tr_m(\rho) \psum{p} tr_m{\sigma}}$. It's easy to show that $\rho'_m \psum{q} \sigma'_m = \nu'_m$, from which it follows that
	\[
		\singleton{\conf{\nu'_m, P'[\sfrac{m}{y}], R}} \ \rel \ \left(\singleton{\conf{\rho'_m, P'[\sfrac{m}{y}], R}} \psum{q} \singleton{\conf{\sigma'_m, P'[\sfrac{m}{y}], R}}\right)
	\]
	and $\Delta' \ Cv(\rel)  \ \left(\Theta'_\rho \psum{p} \Theta'_\sigma\right)$.

	The $\rulename{OQMeas}$ case is identical, and all the other cases of $\tauarrow$ and $\longsquiggly_\pi$ are trivial, as they do not modify the quantum state.

	For the third condition, we must prove that if $\Theta \longsquiggly_\pi \Theta'$, then $\Delta \longsquiggly_\pi \Delta'$ for some $\Delta' \sim_{cs} Cv(\rel) \sim_{cs} \Theta'$. Notice that $\conf{\rho, P, R} \longsquiggly_\pi \bot$ if and only if $\conf{\sigma, P, R} \longsquiggly_\pi \bot$, so we have that either $\Theta \longsquiggly_\pi \bot$ or $\Theta \longsquiggly_\pi \Theta'$ with $\bot \not\in \lceil\Theta' \rceil$. In the first case, also $\Delta \longsquiggly_\pi \bot$, and the condition is satisfied.
	For the second case, we say $\Theta \longsquiggly_\pi$ if there exists a $\Theta'$ such that $\Theta \longsquiggly_\pi \Theta'$ and $\bot \not\in \lceil\Theta' \rceil$. We will show that, if $\Theta \longsquiggly_\pi$, there exist $\hat{\Theta}, \hat{\Delta}$ such that $\Theta \longsquiggly_\pi \hat{\Theta}$, $\Delta \longsquiggly_\pi \hat{\Delta}$ and $\hat{\Delta} Cv(\rel) \hat{\Theta}$. From this, since $\Theta$ is deterministic according to \autoref{sum of deterministic is deterministic}, it must be that for any $\Theta \longsquiggly_\pi \Theta'$ we have $\hat{\Delta} \sim_{cs} Cv(\rel) \sim_{cs} \Theta'$.

	Assume $ \singleton{\conf{\rho, P, R}} \psum{p} \singleton{\conf{\sigma, P, R}} \longsquiggly_\pi$. To prove the existence of $\hat{\Theta}$ and $\hat{\Delta}$, in the case $\pi = \diamond$, we will proceed by induction on the syntax of $P$; in the case $\pi \neq \diamond$, we will proceed by induction on the syntax of $R$.

	Suppose that $\pi = \diamond$. If $P = \tau.P'$, the only possible transition is when $\hat{\Theta} = \singleton{\conf{\rho, P', R}} \psum{p} \singleton{\conf{\sigma, P', R}}$, and we have the transition $\singleton{\conf{\nu, \tau.P', R}} \longsquiggly_\diamond \singleton{\conf{\nu, P', R}} = 	\hat{\Delta}$, with $\hat{\Delta} \rel 	\hat{\Theta}$.

	If $P = \sop{E}{\tilde{x}}.P'$ or $P = \meas{\tilde{x}}{y}.P$, there is only one possible $\hat{\Theta}$ and $\hat{\Delta}$, and the proof proceeds in the same way as seen for the previous direction of bisimulation.

	If $P = P_1 + P_2$,  at least one between $P_1$ or $P_2$ is not in deadlock.
	Suppose that $P_1$ is not in deadlock, then there exists a transition
	\[
		\singleton{\conf{\rho, P_1, R}} \psum{p} \singleton{\conf{\sigma, P_1, R}} \longsquiggly_\diamond \hat{\Theta}
	\]
	For the inductive hypothesis, we have that $
		\singleton{\conf{\nu, P_1, R}} \longsquiggly_\diamond \hat{\Delta} $
	with $\hat{\Delta} \ Cv(\rel) \ \hat{\Theta}$.
	If $P_1$ is in deadlock, then $P_2$ must not, and the proof is symmetrical.

	If $P = P_1 \parallel P_2$, suppose that $P_1$ is not in deadlock, then there exists a transition
	\[
		\singleton{\conf{\rho, P_1, R}} \psum{p} \singleton{\conf{\sigma, P_1, R}} \longsquiggly_\diamond \mathring{\Theta}
	\]
	and a transition $\Theta \longsquiggly_\diamond \hat{\Theta} = \mathring{\Theta} \parallel P_2$.
	For the inductive hypothesis, we have that $\singleton{\conf{\nu, P_1, R}} \longsquiggly_\diamond \mathring{\Delta} $
	with $\mathring{\Delta} \ Cv(\rel) \ \mathring{\Theta}$, from which it follows that
	\[\hat{\Delta} = \mathring{\Delta} \parallel P_2 \quad Cv(\rel) \quad \mathring{\Theta} \parallel P_2 = \hat{\Theta}\]

	If $P_1$ is in deadlock and $P_2$ is not, then the proof is symmetrical. If both $P_1$ and $P_2$ are in deadlock, then there must be a synchronization, i.e.
	$P_1 \parallel P_2 \equiv (c!v + S) \parallel (c?x.P') + Q$. But then there exist the transitions $\Theta \longsquiggly_\diamond \hat{\Theta}$ with
	\[
		\hat{\Theta} = \singleton{\conf{\rho, P'[\sfrac{v}{x}], R}} \psum{p} \singleton{\conf{\sigma, P'[\sfrac{v}{x}], R}}
	\]
	and the transition $\Delta \longsquiggly_\diamond \hat{\Delta}$ with
	\[
		\hat{\Delta} = \singleton{\conf{\nu, P'[\sfrac{v}{x}], R}}
	\]

	If $P = P \setminus c$  or $P = \ite{e}{P_1}{P_2}$, the required property follows trivially from the inductive hypothesis.

	Suppose that $\pi \neq \diamond$, we proceed by induction on $R$. If $R = \sop{E}{\tilde{x}}.R'$ or $R = \meas{\tilde{x}}{y}.R$, the proof proceeds in the same way as before.

	If $R$ is a sum of receptions, then $R \equiv c?x.R_1 + R_2$ and it must be $P
		\equiv ((c!v + S) \parallel Q) \setminus D$; if $R = c!e$, then it must be $P
		\equiv (((c?x . P') + P'') \parallel Q) \setminus D$. In both cases, there exists
	two specific $\hat{\Theta}, \hat{\Delta}$ such that $\hat{\Theta} \ Cv(\rel) \
		\hat{\Delta}$, as seen before for the synchronization  between processes.

	If $R = R_1 \expar R_2$ and $\Theta \longsquiggly_{\ell \cdot \pi'}$, then the required property follows from the inductive hypothesis, as seen before for process parallelism. If $\Theta \longsquiggly_{r \cdot \pi'}$, the case is symmetrical.

	If $R= \ite{e}{R_1}{R_2}$, the required property follows trivially from the inductive hypothesis.
\end{proof}

Consider now the refinement relation $\preceq$, defined as $P' \preceq P$ if $P'$ can be obtained from $P$ by substituting some occurrence of $Q + Q'$ with either $Q$, $Q'$ or $\ite{e}{Q}{Q'}$ for some $e$.
We extend the relation to configurations writing $\conf{\rho', P'} \preceq \conf{\rho, P}$ and $\conf{\rho', P', R'} \preceq \conf{\rho, P, R}$ when $\rho' = \rho$, $P' \preceq P$, and $R' = R$.
Moreover, we lift $\preceq$ to distributions by linearity and imposing $\bot \preceq \Delta$ for any $\Delta$.

\subsection{Proof of \autoref{thm:nondetVSite}}
To prove~\autoref{thm:nondetVSite} we start from some auxiliary lemmas.

\begin{lemma}\label{thm:nondetVSitelm0}
	Let $P' \preceq P$, if $P' \equiv Q'$ then $P \equiv Q$ for some $Q$ such that $Q' \preceq Q$.
\end{lemma}
\begin{proof}
	Trivial by cases on the rules for $\equiv$.
\end{proof}

\begin{lemma}\label{thm:nondetVSitelm1}
	Let $P' \preceq P$, if $\conf{\rho, P'} \tauarrow \Delta'$ then $\conf{\rho, P} \tauarrow \Delta$ for some $\Delta$ such that $\Delta' \preceq \Delta$.
\end{lemma}
\begin{proof}
	Consider the case $\Delta' \neq \bot$.
	We proceed by induction on the rules for $\conf{\rho, P'} \tauarrow \Delta'$.

	If the rule is \rulename{Tau}, then $P' = \tau.Q_1' + Q_2'$, with $\Delta' = \singleton{\conf{\rho, Q_1'}}$ and can only be the refinement of $P = \tau.Q_1 + Q_2$ for $Q_i' \preceq Q_i$.
	Then $\conf{\rho, P} \tauarrow \singleton{\conf{\rho, Q_1}}$, and the refinement holds by definition.

	The same applies to \rulename{Restrict}, \rulename{QOP} and \rulename{QMeas} by noticing that $P'\setminus c \preceq P$ only if $P = P'' \setminus c$, and that $P' \preceq P$ implies $P'[v/x] \preceq P[v/x]$ for any $v$ and $x$.

	Consider \rulename{Par}, then $P' = Q_1' \parallel Q_2'$, with $\Delta' = \Theta' \parallel Q_2'$ for some $\Theta'$ such that $\conf{\rho, Q_1'} \tauarrow \Theta'$.
	Notice that $P$ must be equal $Q_1 \parallel Q_2$ for some $Q_1$ and $Q_2$ such that $Q_i' \preceq Q_i$.
	By induction hypothesis, $\conf{\rho, Q_1} \tauarrow \Theta$ for some $\Theta$ such that $\Theta' \preceq \Theta$, and thus, by \rulename{Par} rule, $\conf{\rho, Q_1 \parallel Q_2} \tauarrow \Theta \parallel Q_2$, and $\Theta' \parallel Q_2' \preceq \Theta \parallel Q_2$ by definition.

	Consider \rulename{Congr} and assume $P' \equiv Q'$, $\conf{\rho, Q'} \tauarrow \Theta'$ and $\Theta' \equiv \Delta'$.
	By~\autoref{thm:nondetVSitelm0}, there exists some $Q$ such that $P \equiv Q$ and $Q' \preceq Q$.
	Then, by induction hypothesis, $\conf{\rho, Q} \tauarrow \Theta$ with $\Theta' \preceq \Theta$.
	From $\Theta' \equiv \Delta'$ and $\Theta' \preceq \Theta$, we know by~\autoref{thm:nondetVSitelm0} that $\Theta \equiv \Delta$ for some $\Delta$ such that $\Delta' \preceq \Delta$.
	Then $\conf{\rho, P} \tauarrow \Delta$ by applying \rulename{Congr}.

	Finally, consider the case in which $\Delta' = \bot$.
	Then, $\conf{\rho, P} \tauarrow \Delta$ either for $\Delta = \bot$ or for some $\Delta \neq \bot$, and in both cases $\bot \preceq \Delta$.
\end{proof}

\begin{lemma}\label{thm:nondetVSitelm2}
	Let $P' \preceq P$, if $\conf{\rho, P', R} \longsquiggly_\pi \Delta'$ then $\conf{\rho, P, R} \longsquiggly_\pi \Delta$ for some $\Delta$ such that $\Delta' \preceq \Delta$.
\end{lemma}
\begin{proof}
	Consider the case in which $\Delta' \neq \bot$.
	We proceed by induction on the rules for $\conf{\rho, P', R} \longsquiggly_\pi \Delta'$.

	Rules \rulename{OQOp}, \rulename{OQMeas}, \rulename{ParL} and \rulename{ParL} are trivial, since the rule is applicable for any process $P$.

	Consider \rulename{Input}, then $P' = (c!v + P_1') \parallel P_2' \setminus D$ and $R = c?x.R_1 + R_2$ with $c \notin D$.
	Moreover, $\pi = \epsilon$ and $\Delta' = \singleton{\conf{\rho, P_2' \setminus D, R_1[v/x]}}$.
	Notice that $P'$ can only be the refinement of $P = (c!v + P_1) \parallel P_2 \setminus D$ for $P_i' \preceq P_i$.
	Then the result holds by applying \rulename{Input} for obtaining $\conf{\rho, P, R} \longsquiggly_\pi \singleton{\conf{\rho, P_2 \setminus D, R_1[v/x]}}$.

	The proof for \rulename{Output} is the same, and follows from the fact that $Q' \preceq Q$ implies $Q'[v/x] \preceq Q[v/x]$ for any $v$ and $x$.

	Consider \rulename{process} and assume $\conf{\rho, P'} \tauarrow \Delta'$.
	Then, by~\autoref{thm:nondetVSitelm1}, $\conf{\rho, P} \tauarrow \Delta$ with $\Delta' \preceq \Delta$.
	We can thus apply \rulename{process} to derive $O[\conf{\rho, P}] \longsquiggly_\diamond O[\Delta]$, and $O[\Delta'] \preceq O[\Delta]$ holds by definition.

	Consider \rulename{Congr} and assume $P' \equiv Q'$, $R \equiv_O S$, $\conf{\rho, Q', S} \longsquiggly_\pi \Theta'$ and $\Theta' \equiv_O \Delta'$.
	From~\autoref{thm:nondetVSitelm0},  $P \equiv Q$ such that $Q' \preceq Q$, and thus, by induction hypothesis, $\conf{\rho, Q, S} \longsquiggly_\pi \Theta$ with $\Theta' \preceq \Theta$.
	Hence, from~\autoref{thm:nondetVSitelm0} and by definition of $\preceq$, a distribution $\Delta$ exists such that $\Theta \equiv \Delta$ and $\Delta \preceq \Delta'$.
	We can thus apply \rulename{Congr} to derive $\conf{\rho, P, R} \longsquiggly_\pi \Delta$.

	Finally, consider $\Delta' = \bot$.
	Then, $\conf{\rho, P, R} \longsquiggly_\pi \Delta$ either for $\Delta = \bot$ or for some $\Delta \neq \bot$, and in both cases $\bot \preceq \Delta$.
\end{proof}

\nondetVSite*
\begin{proof}
	By~\autoref{thm:nondetVSitelm2} and decomposability of $\longsquiggly_{\pi}$.
\end{proof}
