# Supplementary material for: Quantum Bisimilarity is a Congruence under Physically Admissible Schedulers
Source: arXiv:2408.15087 source file (2024-08-27)
Supplement: Supplementary file 2 [file appendix_properties.tex]

\thmchinese*
\begin{proof}
 To prove the first point, suppose $\conf{\rho, P, \nil} \sim_{cs} \conf{\sigma, Q, \nil}$, with $\rho, \sigma \in \hilbert_{\tilde{q},\tilde{p}}$ and $\tilde{p} \vdash P$, $\tilde{p} \vdash Q$.  For any superoperator $\mathcal{TS}(\hilbert_{\tilde{q}})$ 
 we can construct a context 
 \[
 O[\blank] = [\blank] \parallel \sop{E}{{\tilde{q}}}.(a!0 \parallel c!\tilde{q})
 \] where $a$ is a fresh channel. We know that $O[\conf{\rho, P, \nil}]$ and $O[\conf{\sigma, Q, \nil}]$ are bisimilar, and $O[\conf{\rho, P, \nil}]$ can evolve in $\conf{\sop[\tilde{q}]{E}{\rho}, P, a!0 \parallel c!\tilde{q} \parallel \nil}$.
  Then $O[\conf{\sigma, Q, \nil}]$ must evolve in $\conf{\sop[\tilde{q}]{E}{\sigma}, Q, a!0 \parallel c!\tilde{q} \parallel \nil}$, because it must match the $\downarrow_a$ barb, and $a$ is fresh. So we have that  
\[\conf{\sop[\tilde{q}]{E}{\rho}, P, a!0 \parallel c!\tilde{q} \parallel \nil} \sim_{cs} 
  \conf{\sop[\tilde{q}]{E}{\sigma}, Q, a!0 \parallel c!\tilde{q} \parallel \nil}
\]
and from this it follows 
\[ \conf{\sop[\tilde{q}]{E}{\rho}, P, \nil} \sim_{cs} 
  \conf{\sop[\tilde{q}]{E}{\sigma}, Q, \nil}
\] simply by contradiction: if there was a context capable of distinguishing $\conf{\sop[\tilde{q}]{E}{\rho}, P, \nil}$ from $\conf{\sop[\tilde{q}]{E}{\rho}, P, \nil}$ then there would be a context able to distinguish also $\conf{\sop[\tilde{q}]{E}{\rho}, P, a!0 \parallel c!\tilde{q} \parallel \nil}$ from $\conf{\sop[\tilde{q}]{E}{\sigma}, Q, a!0 \parallel c!\tilde{q} \parallel \nil}$.

To prove the second point we proceed by contradiction, supposing  $\conf{\rho, P, \nil} \sim_{cs} \conf{\sigma, Q, \nil}$  and $tr_{\tilde{p}}(\rho) \neq tr_{\tilde{p}}(\sigma)$, with $\rho, \sigma \in \hilbert_{\tilde{q}, \tilde{p}}$ and $\tilde{p} \vdash P$, $\tilde{p} \vdash Q$.
 If $\ptrace{p}{\rho} \neq \ptrace{p}{\sigma}$, then there exists a measurement $M_{\tilde{q}} = \{M_1, \ldots ,M_m\}$ that distinguishes them, i.e.\ such that $p_m(\ptrace{p}{\rho}) = tr(M_m \ptrace{p}{\rho} M_m^\dagger) \neq tr(M_m \ptrace{p}{\sigma} M_m^\dagger) = p_m(\ptrace{p}{\sigma})$ for some $m$. But for \autoref{ptrace drops sop}, the same probabilities arise also from the measurement $M_{\tilde{q}\tilde{p}} = \{M_1 \otimes I_{\tilde{p}}, \ldots , M_m \otimes I_{\tilde{p}}\}$, that  can therefore distinguish the whole state $\rho$ from $\sigma$. So, taken the context 
\begin{align*}
O[\blank] =& [\blank] \parallel \meas{\tilde{q}}{x}. \\
&\nil_{\tilde{q}} \parallel \ite{x = 1}{c_1!0}{\ldots} \\
&\qquad\quad\ite{x = m-1}{c_{m-1}!0}{c_m!0}
\end{align*} 
where $c_1 \ldots c_m$ are fresh channels, we have that $O[\conf{\rho, P, \nil}]$ should be bisimilar to $O[\conf{\sigma, Q, \nil}]$. 
But 
\[O[\conf{\rho, P, \nil}] \longsquiggly_r \sum_m \distelem{p_m(\rho)} \conf{\rho_m, P, \nil \parallel c_m!0}\]
and $O[\conf{\sigma, Q, \nil}]$ can perform only the transition \[O[\conf{\sigma, Q, \nil}] \longsquiggly_r \sum_m \distelem{p_m(\sigma)} \conf{\sigma_m, Q, \nil \parallel c_m!0}\] to match the barbs, but we know that $p_m(\rho) \neq p_m(\sigma)$ for at least one $m$.
\end{proof}

In order to prove \autoref{thm:discarded}, we need an additional lemma.

\begin{lemma}\label{ptrace preserves arrow}
Assume that $\Delta$ is a distribution such that $\ptrace{q}{\Delta}$ is well-defined. Then, for $O[\blank]$ we have
\[ O[\Delta] \longsquiggly_\pi \Delta' \text{ if and only if } O[\ptrace{q}{\Delta}] \longsquiggly_\pi \ptrace{q}{\Delta'}
\]
\end{lemma}
\begin{proof}
We will prove that, for any $\iconf \in \confbot$
\[
\singleton{\mathcal{C}}\longsquiggly_\pi \Delta' \text{ if and only if } \ptrace{q}{\singleton{\mathcal{C}}} \longsquiggly_\pi \ptrace{q}{\Delta'}
\]
from which the desired lemma follows easily  by linearity.

We will proceed by induction on $\singleton{\mathcal{C}}\longsquiggly_\pi \Delta'$. First, if $\iconf = \bot$, then the property follows from the definitions of $O[\bot]$ and $\ptrace{q}{\bot}$. Otherwise, notice that $disc(\tilde{q})$ is a deadlock process that cannot take part in any synchronization. The only interesting base cases are $\rulename{QOp}$, $\rulename{QMeas}$, $\rulename{OQOp}$ and $\rulename{OQMeas}$, when the process (or the observer) modifies the quantum state. We will deal only with the process, as the proof for observer is the same. All the other rules of $\rightarrow$ and $\longsquiggly$ are trivial, as they do not modify the quantum state. 

Assume that \[\singleton{\conf{\rho, (\sop{E}{\tilde{x}}.P + Q \parallel \nil_{\tilde{q}}), R}} \rightarrow \singleton{\conf{\sop[\tilde{x}]{E}{\rho}, (P \parallel \nil_{\tilde{q}}), R}}\]
with $\sop[\tilde{x}]{E}{\rho} = (\mathcal{E}\otimes \mathcal{I}_{\tilde{y}} \otimes \mathcal{I}_{\tilde{q}})(\rho)$, where $\tilde{y}$ are all the qubits not in $\tilde{x}$ nor in $\tilde{q}$, and $ \mathcal{I}_{\tilde{y}}$ is the identity superoperator on said qubits.
Then we also have \[\singleton{\conf{\ptrace{q}{\rho},(\sop{E}{\tilde{x}}.P + Q), R}} \rightarrow \singleton{\conf{\sop[\tilde{x}]{E}{\ptrace{q}{\rho}}, P, R}}\]
with $\sop[\tilde{x}]{E}{\ptrace{q}{\rho}} = (\mathcal{E}\otimes \mathcal{I}_{\tilde{y}}) (\ptrace{q}{\rho})$.
  From \autoref{ptrace drops sop}, we have 
  \[(\mathcal{E}\otimes \mathcal{I}_{\tilde{y}}) (\ptrace{q}{\rho}) = \ptrace{q}{(\mathcal{E}\otimes \mathcal{I}_{\tilde{y}} \otimes \mathcal{I}_{\tilde{q}})(\rho)}\]
  and we conclude  
	\[\singleton{\conf{\sop[\tilde{x}]{E}{\ptrace{q}{\rho}}, P, R}} = \ptrace{q}{\singleton{\conf{\sop[\tilde{x}]{E}{\rho}, (P \parallel \nil_{\tilde{q}}), R}}}\]
 The other direction is similar.
	
	The $\rulename{QMeas}$ case is also similar: \autoref{ptrace drops sop} implies $tr\left(\ptrace{q}{\sop[\tilde{x}, m]{M}{\rho}}\right) = tr\left(\sop[\tilde{x}, m]{M}{\ptrace{q}{\rho}}\right)$, so $\Delta'$ and $\ptrace{q}{\Delta'}$ have the same probabilities.
\end{proof}

We can now prove that distribution bisimilarity is closed for additional discarded qubits.

\bisimilaritydiscarded*
\begin{proof}
We need to show that 
\[\rel = \left\{(\Delta, \Theta) \mid  \ptrace{q}{\Delta} \sim_{cs} \ptrace{q}{\Theta}\right\}
\]
is a distribution bisimulation. Notice that if $\Sigma \vdash \Delta, \Theta$, then $\Sigma \setminus \tilde{q} \vdash \ptrace{q}{\Delta}, \ptrace{q}{\Theta}$.

For the first condition, observe that $\Delta \downarrow^p_b$ if and only if $\ptrace{q}{\Delta} \downarrow^p_b$, since the partial trace operation is linear and the process $\nil_{\tilde{q}}$ does not express any barb.

For the second condition, it is sufficient to notice that $\ptrace{q}{O[\Delta]} = O[\ptrace{q}{\Delta}]$ for any context $O[\blank]$. Then, we have that if $O[\Delta] \longsquiggly_\pi \Delta'$, then from \autoref{ptrace preserves arrow} we know that $\ptrace{q}{O[\Delta]} = O[\ptrace{q}{\Delta}] \longsquiggly_\pi \ptrace{q}{\Delta'}$, and then $O[\ptrace{q}{\Theta}] \longsquiggly_\pi \Theta'' \sim_{cs} \ptrace{q}{\Delta'}$ and $O[\Theta] \longsquiggly_\pi \Theta'$ such that $\Theta'' = \ptrace{q}{\Theta'}$. The third condition is symmetric.
\end{proof}

\uptocv*
\begin{proof}
Soundness follows from compatibility, proven in~\autoref{thm:cvcomp}, as shown in~\cite{sangiorgienhancements2011}.
\end{proof}
