# Supplementary material for: Quantum Bisimilarity is a Congruence under Physically Admissible Schedulers
Source: arXiv:2408.15087 source file (2024-08-27)
Supplement: Supplementary file 3 [file appendix_quantum_proof_preliminaries.tex]

\anote{Serve?}
\red{\begin{lemma}\label{ptrace drops sop}
Let $\rho \in \density{\hilbert_{\tilde{p}} \otimes \hilbert_{\tilde{q}}}$, with $\tilde{p} = p_0 \ldots p_{n-1}$ and $\tilde{q} = q_0 \ldots q_{m-1}$.
 Then, for any two superoperator $\mathcal{E}_{\tilde{p}} \in \soset{\hilbert_{\tilde{p}}}$
 and $\mathcal{F}_{\tilde{q}} \in \tsoset{\hilbert_{\tilde{q}}}$
\[
 \ptrace{q}{(\mathcal{E}_{\tilde{p}} \otimes \mathcal{F}_{\tilde{q}}) (\rho)} = \sop[\tilde{p}]{E}{\ptrace{q}{\rho}}
\]
\end{lemma}
\begin{proof}
  The density operator $\rho$ is described in the form $\rho = \sum_{ijkl} \rho_{ij,kl}\ketbra{ij}{kl}$, where $i,k$ are elements of some orthonormal basis of $\hilbert_{\tilde{p}}$ and $j,l$ of $\hilbert_{\tilde{q}}$
  \begin{align*}
    \ptrace{q}{(\mathcal{E}_{\tilde{p}} \otimes \mathcal{F}_{\tilde{p}})\rho} &= \sum_{ijkl}\rho_{ij,kl}\ptrace{q}{\mathcal{E}_{\tilde{p}}(\ketbra{i}{k}) \otimes \mathcal{F}_{\tilde{q}}(\ketbra{j}{l})} \\
    &= \sum_{ijkl}\rho_{ij,kl}\,\mathcal{E}_{\tilde{p}}(\ketbra{i}{k})\tr(\mathcal{F}_{\tilde{q}}\ketbra{j}{l}) \\
    &= \mathcal{E}_{\tilde{p}}\left(\sum_{ijkl}\rho_{ij,kl}\ketbra{i}{k}\tr(\ketbra{j}{l})\right) \\
    &= \mathcal{E}_{\tilde{p}}\left(\sum_{ijkl}\rho_{ij,kl}\ptrace{q}{\ketbra{ij}{kl}}\right) \\
    &= \mathcal{E}_{\tilde{p}}\left(\ptrace{q}{\sum_{ijkl}\rho_{ij,kl}\ketbra{ij}{kl}}\right)
    = \mathcal{E}_{\tilde{p}}(\ptrace{q}{\rho}) \qedhere
  \end{align*}
\end{proof}}
